# Supplementary material for: DnD: Dense Depth Estimation in Crowded Dynamic Indoor Scenes
Source: arXiv:2108.05615 source file (2021-08-12)

# RGB Input

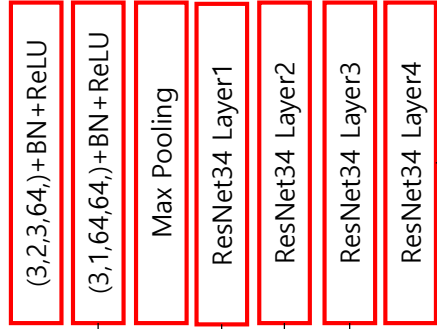

# Projected Depth

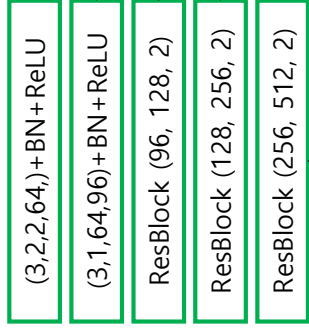

$\oplus$  : Addition    $\odot$  : Concatenation   BN: Batch Normalization

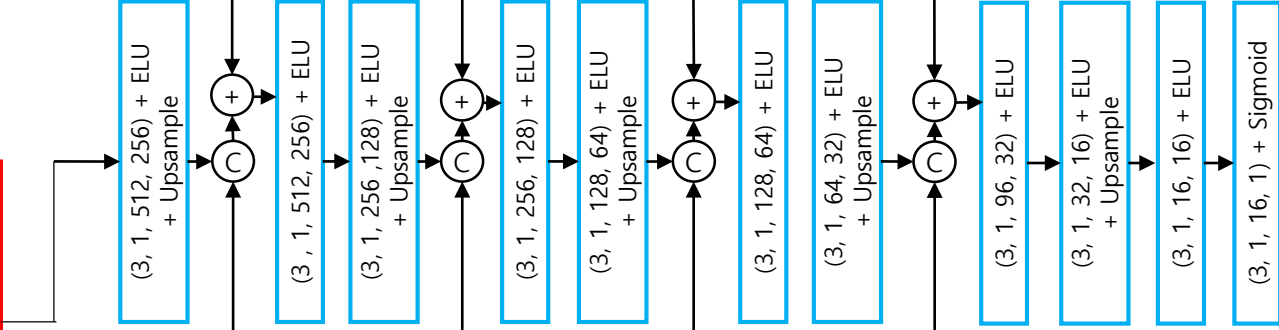

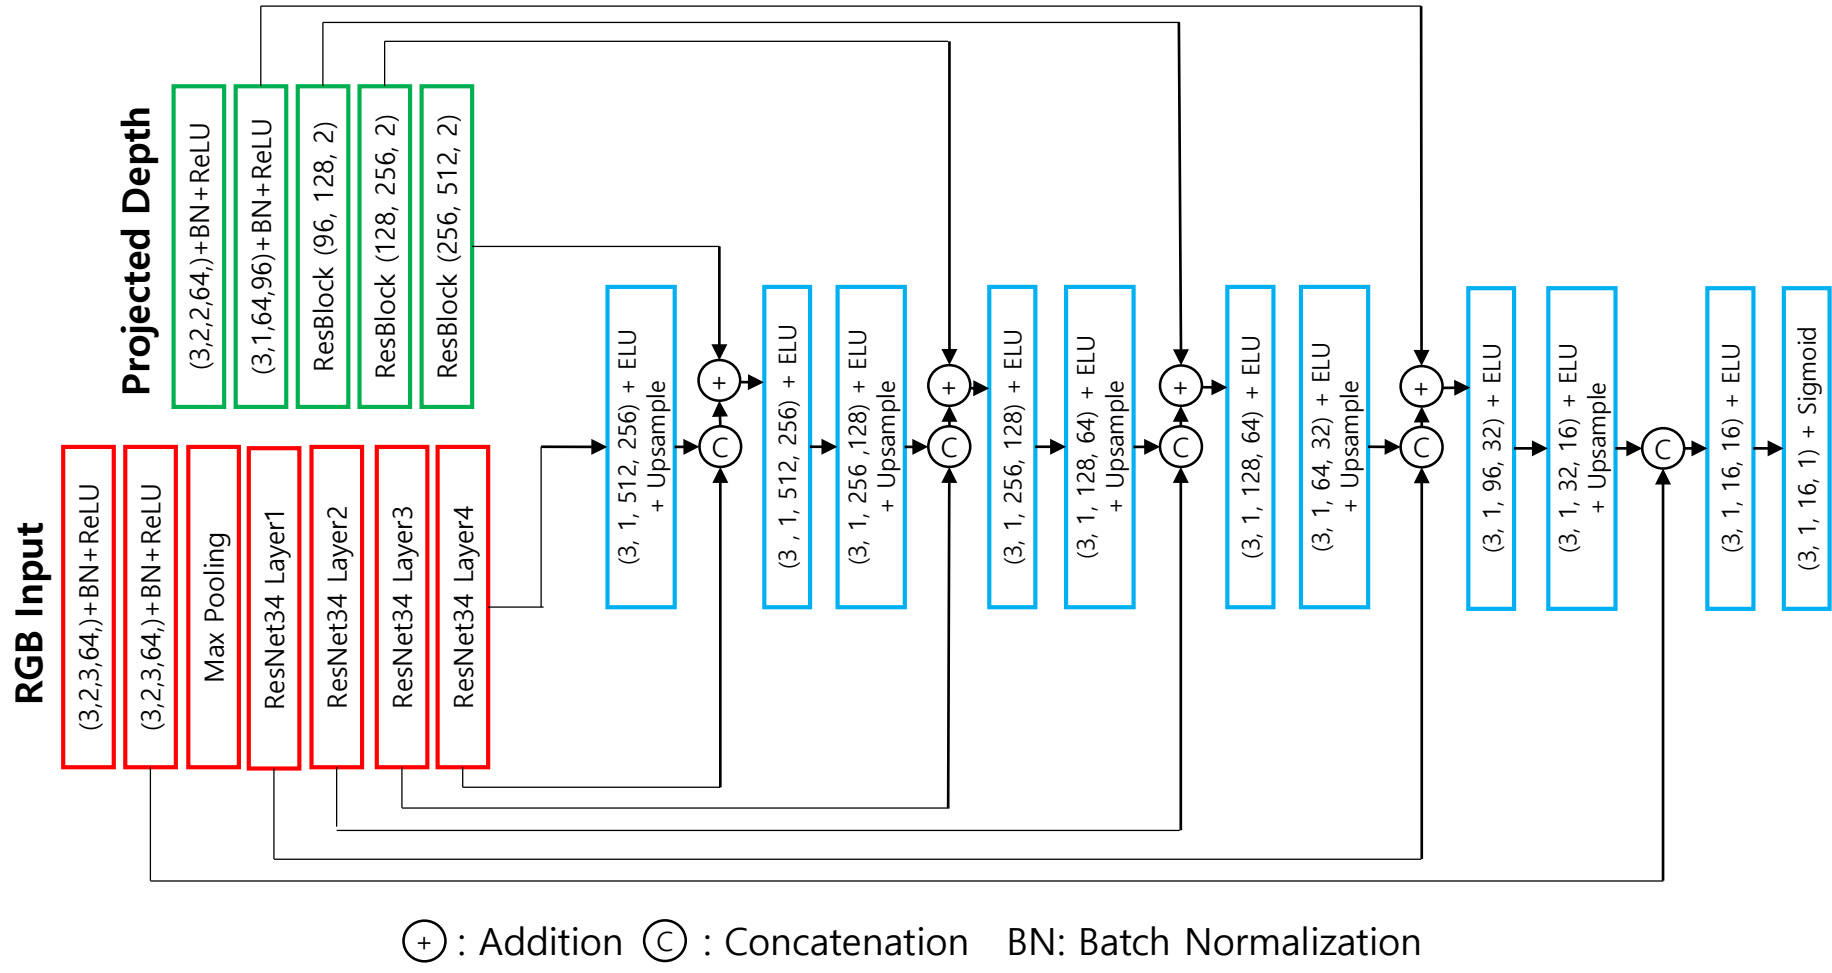

Supplement: Supplementary file 1 [file model.pdf]
