# Supplementary material for: DnD: Dense Depth Estimation in Crowded Dynamic Indoor Scenes
Source: arXiv:2108.05615 source file (2021-08-12)

*Flow*

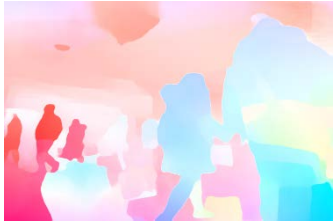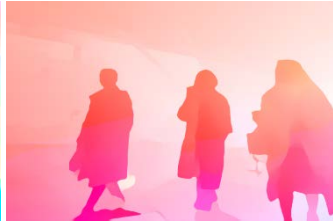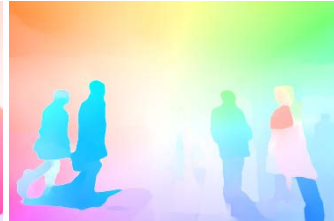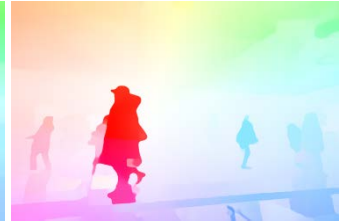

$I'_t$

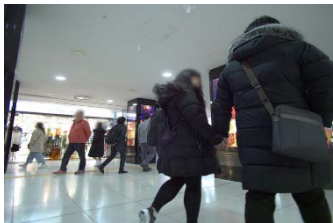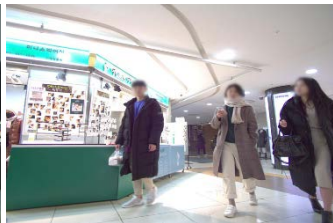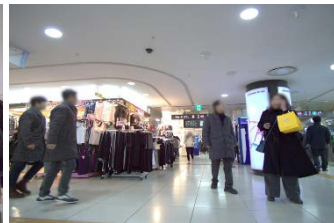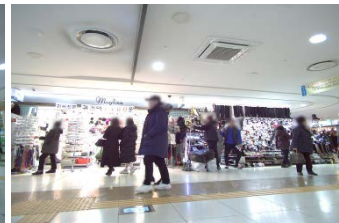

$I'_t$

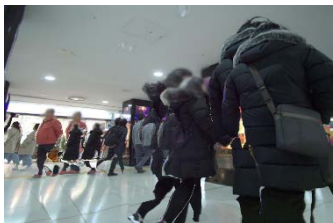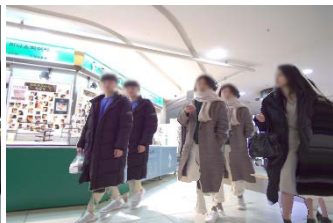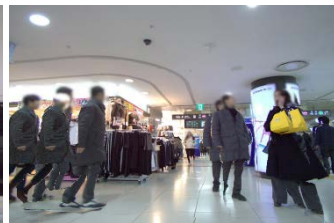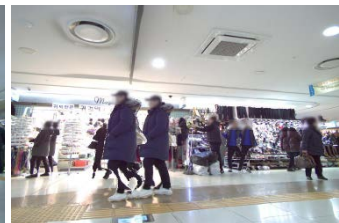

$I_t$

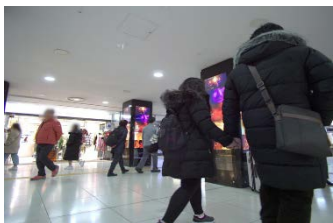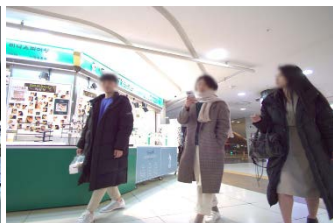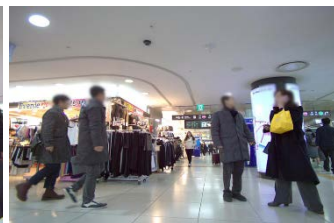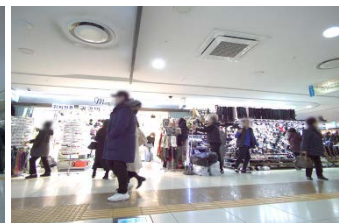

*Flow*

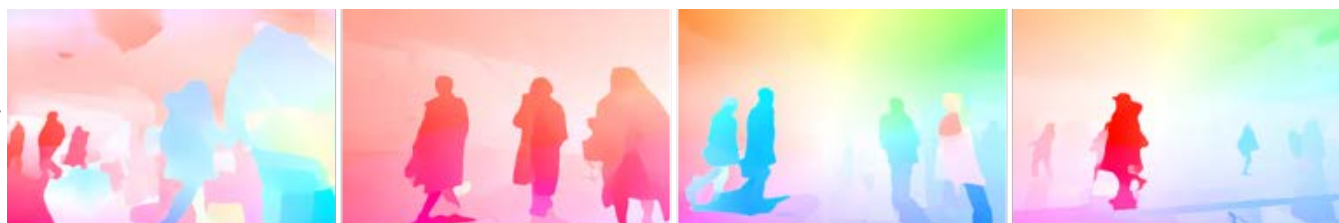

$I_t'$

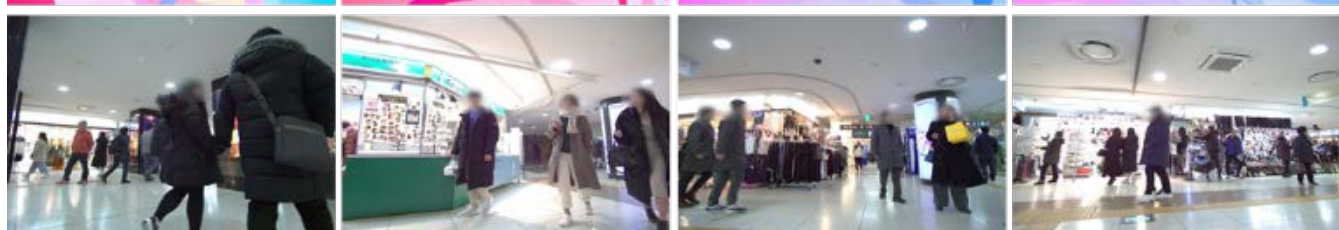

$I_t'$

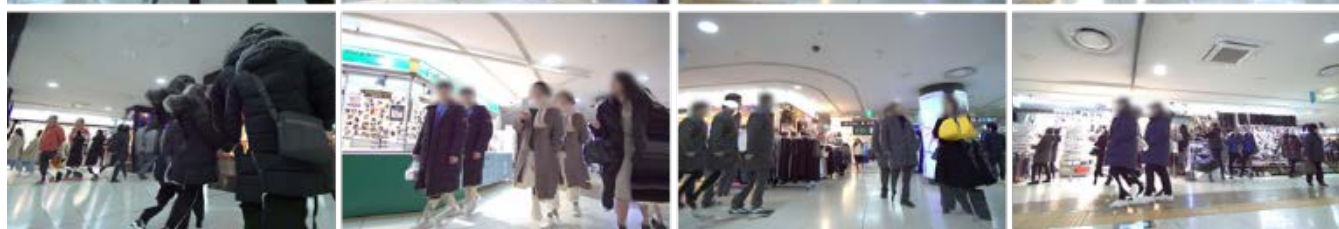

$I_t$

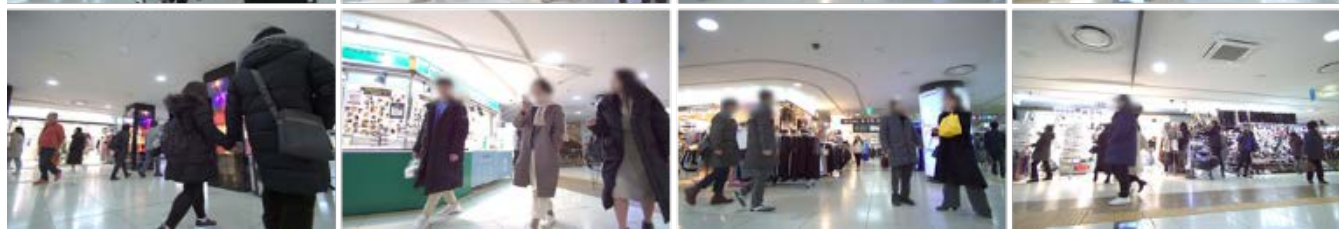

Supplement: Supplementary file 2 [file supple_flow.pdf]
